# Supplementary material for: An Isoperimetric Inequality for Fundamental Tones of Free Plates
Source: arXiv:1004.0016 source file (2010-03-31)
Supplement: Supplementary file 1 [file ubappendix.tex]

\chapter{The unit ball under compression (to be revised)}\label{ubappendix}
In this chapter, we complete our classification of the solutions to the free plate equation on the unit ball for all values of $\tau$.

\textbf{Still To Do:} This section needs revising. The material in this chapter needs to be discussed more thoroughly and some details should be added.

\subsection*{Zero eigenvalues}
When $\omega = 0$, \eqref{maineq} can be factored as
\begin{equation}
\Delta(\Delta-\tau)u = 0.
\end{equation}
From the Rayleigh quotient we see that the only solutions for $\omega = 0$ with  $\tau > 0 $ are constant. For $\tau\leq 0 $, our solutions will have the form
\[
u(x)=\left(mr + b +C j_l(\sqrt{|\tau|}r)\right)Y_l(\hat{\theta}),
\]
for some real constant $C$.
\subsection*{Negative eigenvalues}
Again, we note that for $\tau\geq 0$, all terms in the Rayleigh quotient are nonnegative, and so there are no negative eigenvalues when $\tau \geq 0$. When $\tau < 0$, there are three possibilities for factoring \eqref{maineq}, depending on the relative values of $\tau$ and $\omega$.

When $0>\omega>-\tau^2/4$, the eigenvalue equation factors as
\[
(\Delta+a^2)(\Delta+b^2)u = 0,
\]
with $a$, $b$ real and positive, $\omega=-a^2b^2$ and $\tau = -a^2-b^2$. Our solutions will then be of the form
\[
u(x)=\Big(j_l(ar)+\gamma j_l(br)\Big)Y_l(\hat{\theta}).
\]

When $\omega=-\tau^2/4$, the eigenvalue equation  factors as
\[
(\Delta+a^2)^2u = 0,
\]
with $a=\sqrt{-\tau/2}$ real and positive. Our solutions will then be of the form
\[
u(x)=\Big(j_l(ar)+\gamma r j_l'(ar)\Big)Y_l(\hat{\theta}).
\]

When $\omega<-\tau^2/4$, the discriminant of $x^2-\tau x-\omega$ is negative and so the eigenvalue equation factors as
\[
(\Delta+c^2)(\Delta+\bar{c}^2)u = 0,
\]
with $c$ nonreal such that $\omega=-|c|^4$ and $\tau=-2\Real{c}$. Our solutions will then be of the form
\[
u(x)=\Big(j_l(cr)+\gamma j_l(\bar{c}r)\Big)Y_l(\hat{\theta}).
\]
